# Supplementary material for: A nano vacuum gauge based on second-order coherence in optical levitation
Source: arXiv:2404.06907 source file (2024-04-10)
Supplement: Supplementary file 1 [file SM.pdf]

# Supplemental Material: A nano vacuum gauge based on second-order coherence in optical levitation

Lyu-Hang Liu,[1,2] Yu Zheng,[1,2,*] Yuan Tian,[1,2] Long Wang,[1,2] Guang-Can Guo,[1,2] and Fang-Wen Sun[1,2,†]

[1] *CAS Key Laboratory of Quantum Information, University of Science and Technology of China, Hefei 230026, China*

[2] *CAS Center for Excellence in Quantum Information and Quantum Physics, University of Science and Technology of China, Hefei 230026, China*

(Dated: March 4, 2024)

## CONTENTS

1. Dynamic of levitated nano-particle's energy 2

1.1. Stochastic equations for energy 2

1.2. Approximate stochastic equations in high vacuum 3

1.3. Power spectrum of energy in high vacuum 4

2. Differences in readings between capacitance gauges and cold cathode gauges 5

* bigz@ustc.edu.cn

† fwsun@ustc.edu.cn

## 1. DYNAMIC OF LEVITATED NANO-PARTICLE'S ENERGY

### 1.1. Stochastic equations for energy

Consider a levitated particle with mass $m$ oscillating in a trap without any feedback process. All the forces on it consist of the trapping force $F_{\text{trap}}$, drag force $F_{\text{damp}}$, stochastic force $F_{\text{therm}}$ driven thermally:

$$\begin{cases} F_{\text{trap}} = -m\omega_0^2 q\left(1+\sum_{i=2}^{n}\xi_i q^{i-1}\right) \\ F_{\text{damp}} = -\Gamma_0 p \\ F_{\text{therm}} = \sqrt{2mk_{\text{B}}T\Gamma_0}\,w(t), \end{cases} \tag{S1}$$

where $q$ specifies the position of the particle, $\omega_0$ is the natural frequency in the harmonic case, $\xi_i$ describes the nonlinear coefficients dependent on the shape of the potential, which quantifies the extent of deviation from a purely harmonic potential. The damping coefficient $\Gamma_0$ arises from a gas of temperature $T$, $p = m\dot{q}$ denotes the momentum of the particle, $k_{\text{B}}$ is the Boltzmann constant and $w(t)$ represents white noise.

These forces yield the stochastic equations of motion for the particle,

$$\begin{cases} dq = \frac{p}{m}dt \\ dp = \left(F_{\text{trap}} + F_{\text{damp}}\right)dt + \sqrt{2m\Gamma_0 k_{\text{B}}T}\,dW. \end{cases} \tag{S2}$$

Here, $W(t)$ is the Wiener process, which satisfies $\langle W(t)\rangle = 0$ and $\langle W(t)W(t')\rangle = min\,(t,t')$. For an infinitesimal interval $dt$, one has $\langle (dW)^2\rangle = dt$. Additionally, the white noise component present in the stochastic force can be regarded as the time derivative of the Wiener process, $w(t) = dW(t)/dt$.

In order to ignore the effect of nonlinearity on the oscillator phase, we now explore the time evolution of the energy generated by the stochastic equations of motion. To avoid multiplicative noise, it would be a preferred approach to consider the square root of the energy rather than the energy itself,

$$\begin{cases} \epsilon\,(q,p) = \sqrt{E\,(q,p)} \\ E\,(q,p) = m\omega_0^2\left(\frac{1}{2}q^2 + \sum_{i=2}^{n}\frac{\xi_i}{i+1}q^{i+1}\right) + \frac{p^2}{2m}. \end{cases} \tag{S3}$$

Note that the conservative forces, including those due to the shape of the potential, make no contribution to the energy change. And one can obtain $\dfrac{\partial E}{\partial t} = -F_{\mathrm{trap}}\dfrac{\partial q}{\partial t} + \dfrac{p}{m}\dfrac{\partial p}{\partial t} = \dfrac{pF_{\mathrm{damp}}}{m}$. According to Ito's formula, the stochastic equations for $\epsilon$ can be described as:

$$\mathrm{d}\epsilon = \left[\frac{pF_{\mathrm{damp}}}{2m\epsilon} + \frac{\Gamma_0 k_{\mathrm{B}}T}{2\epsilon}\left(1 - \frac{p^2}{2m\epsilon^2}\right)\right]\mathrm{d}t + \frac{p}{2m\epsilon}\sqrt{2m\Gamma_0 k_{\mathrm{B}}T}\mathrm{d}W. \tag{S4}$$

### 1.2. Approximate stochastic equations in high vacuum

Equation (S4) explicitly depends on the position and momentum of the particle. To remove this dependence and obtain a closed equation depending only on $\epsilon$, we partition the long timescale $t$ into multiple shorter timescale $\tau = 2\pi/\omega$, where $\omega$ is the oscillation frequency. We assume that such a period at low friction (in high vacuum) is shorter than the time for energy relaxation. And the particle undergos an undisturbed harmonic oscillation satisfying $q(t) = R\cos(\omega t + \phi)$, $p(t) = -m\omega R\sin(\omega t + \phi)$ and $R = \sqrt{\dfrac{2}{m}\dfrac{\epsilon}{\omega}}$. In other words, we consider that the energy fluctuations in a period should be insignificant compared to the average energy under this quasi-static assumption.

We obtain the change $\Delta\epsilon$ during the period $\tau$

$$\Delta\epsilon = \int_0^\tau \frac{-\Gamma_0 p^2}{2m\epsilon} + \frac{\Gamma_0 k_{\mathrm{B}}T}{2\epsilon}\left(1 - \frac{p^2}{2m\epsilon^2}\right)\mathrm{d}t + \int_0^\tau \frac{p}{2m\epsilon}\sqrt{2m\Gamma_0 k_{\mathrm{B}}T}\,\mathrm{d}W. \tag{S5}$$

Carrying out the integrals over $t$, the first term in Eq. (S5) yields

$$\Delta\epsilon_1 = -\frac{\epsilon\tau}{2}\Gamma_0 + \frac{\Gamma_0 k_{\mathrm{B}}T\tau}{4\epsilon}, \tag{S6}$$

and the second term in Eq. (S5) represents a stochastic integral resulting from the noise term. As a weighted sum of Gaussian random variables, $\Delta\epsilon_2$ also follows a Gaussian random distribution with its mean and variance

$$\begin{cases} \langle\Delta\epsilon_2\rangle = \sqrt{2m\Gamma_0 k_{\mathrm{B}}T}\displaystyle\int_0^\tau \frac{p}{2m\epsilon}\langle\mathrm{d}W\rangle = 0 \\ \langle(\Delta\epsilon_2)^2\rangle = 2m\Gamma_0 k_{\mathrm{B}}T\displaystyle\int_0^\tau\int_0^\tau \frac{p(t)p'(t)}{4m^2\epsilon^2}\langle\mathrm{d}W\mathrm{d}W'\rangle = \frac{\Gamma_0 k_{\mathrm{B}}T}{2}\tau. \end{cases} \tag{S7}$$

Thus, the random variable $\Delta\epsilon_2$ can be expressed in terms of Wiener process as

$$\Delta\epsilon_2 = \sqrt{\frac{\Gamma_0 k_{\mathrm{B}}T}{2}}W(\tau). \tag{S8}$$

Putting these together, we can obtain the stochastic differential equation for $\epsilon$

$$\mathrm{d}\epsilon = \left(-\frac{\epsilon\Gamma_0}{2} + \frac{\Gamma_0 k_{\mathrm{B}}T}{4\epsilon}\right)\mathrm{d}t + \sqrt{\frac{\Gamma_0 k_{\mathrm{B}}T}{2}}\mathrm{d}W. \tag{S9}$$

According to Ito's formula, substituting $\epsilon$ with $E$ yields the corresponding stochastic differential equation for the energy

$$\mathrm{d}E = (-E\Gamma_0 + \Gamma_0 k_\mathrm{B} T)\,\mathrm{d}t + \sqrt{2E\Gamma_0 k_\mathrm{B} T}\mathrm{d}W. \tag{S10}$$

### 1.3. Power spectrum of energy in high vacuum

We denote the Fourier transformation of $E$ as $\tilde{E} = \mathcal{F}[E]$. Fourier transforming the Eq. (S10) and setting the lower-order term of $E$ as its average $|E|$ gives

$$-i\omega\tilde{E} = -\tilde{E}\Gamma_0 + \Gamma_0 k_\mathrm{B} T\delta(\omega) + \sqrt{2|E|\Gamma_0 k_\mathrm{B} T}\tilde{W}. \tag{S11}$$

We disregard the delta peak at $\omega = 0$, which is $\Gamma_0 k_\mathrm{B} T\delta(\omega)$. The equation above can be solved as

$$\tilde{E} = \frac{\sqrt{2|E|\Gamma_0 k_\mathrm{B} T}}{\Gamma_0 - i\omega}\tilde{W}. \tag{S12}$$

The Wiener process has the property $|W|^2 = 1$, that allows us to obtain the power spectrum of energy

$$S_E(\omega) = |E|^2 = \frac{2|E|\Gamma_0 k_\mathrm{B} T}{\Gamma_0^2 + \omega^2}. \tag{S13}$$

In order to calculate the average of energy, it is necessary to determine the energy distribution of the oscillator in the steady state. The stochastic differential equation Eq. (S10) takes the form of a motion equataion, $\mathrm{d}x = \frac{1}{\upsilon} f(x)\mathrm{d}t + \sqrt{\frac{2k_\mathrm{B}T}{\upsilon}}\mathrm{d}W$, which describes the time evolution of a one-dimensional Brownian particle under the external force $f(x)$ and friction $\upsilon$ at temperature $T$. Consequently, all the conclusions of the overdamped Brownian motion can be applicable. By taking $\upsilon = 4/\Gamma$ and substituting $x$ with $\epsilon$, then we can determine the corresponding force and potential as follows:

$$\begin{cases} \mathrm{d}\epsilon = \frac{1}{\upsilon}\left(-2\epsilon + \frac{k_\mathrm{B}T}{\epsilon}\right)\mathrm{d}t + \sqrt{\frac{2k_\mathrm{B}T}{\upsilon}}\mathrm{d}W \\ f(\epsilon) = -2\epsilon + \frac{k_\mathrm{B}T}{\epsilon} \\ U(\epsilon) = \int -f(\epsilon)\,d\epsilon = \epsilon^2 - k_\mathrm{B}T\ln\epsilon. \end{cases} \tag{S14}$$

Then the distribution of $\epsilon$ can be inferred immediately,

$$P_\epsilon(\epsilon) \propto \exp\left(-\beta_0 U(\epsilon)\right) = \epsilon \exp\left(-\beta_0\epsilon^2\right). \tag{S15}$$

Changing variables from $\epsilon$ to $E$, we can get the probability density function, average and variance of energy,

$$\begin{cases} P_E(E) = \beta_0 \exp\left(-\beta_0 E\right) \\ Avg(E) = k_\mathrm{B}T \quad Var(E) = \left(k_\mathrm{B}T\right)^2 . \end{cases} \tag{S16}$$

Finally, the power spectrum of energy in Eq. (S13) can be approximated as

$$S_E(\omega) = \frac{2\Gamma_0 \left(k_\mathrm{B}T\right)^2}{\Gamma_0^2 + \omega^2}, \tag{S17}$$

which possesses the following properties:

$$\begin{cases} \displaystyle\int_0^\infty \frac{\Gamma_0}{\Gamma_0^2 + \omega^2}\,\mathrm{d}\omega = \frac{\pi}{2} \\ \displaystyle\int_0^\infty S_E(\omega)\,\mathrm{d}\omega = \pi Var(E). \end{cases} \tag{S18}$$

## 2. DIFFERENCES IN READINGS BETWEEN CAPACITANCE GAUGES AND COLD CATHODE GAUGES

The experiments revealed a disruption in the linearity with relative to the reference pressure of both the damping rate and air pressure measurements, when switching from capacitance gauges to cold cathode gauges. To investigate the cause of this gap, we make a comparison of pressure readings between the two types of gauges under identical pressure conditions. The capacitance gauges used in the main manuscript were CMR361 and CMR364 by Pfeiffer Vacuum GmbH, with corresponding ranges of $0.1 \sim 10^3$ mbar and $10^{-4} \sim 1$ mbar, respectively. During the decreasing of pressure, the cold cathode gauge (PKR361 by Pfeiffer Vacuum GmbH) is fully actived when the air pressure below $1 \times 10^{-3}$ mbar. Since the actived pressure of cold cathode gauges is near the lower limit of the range of CMR364, we use a CMR365 (with range of $10^{-5} \sim 0.1$ mbar by Pfeiffer Vacuum GmbH) for comparison with the cold cathode gauge. The cold cathode gauge that used in the main text and a new cold cathode gauge were employed for comparison with capacitance gauge.

Three gauges are connected to the same vacuum chamber. We conducted a series of iterative pressure up and down cycles ranging from $10^{-5}$ to 0.1 mbar, which was repeated five times. Due to potential zero point shift caused by environmental factors, we performed zero adjustments of the capacitance gauge according to the manufacturer's manual before every pressure change cycles.

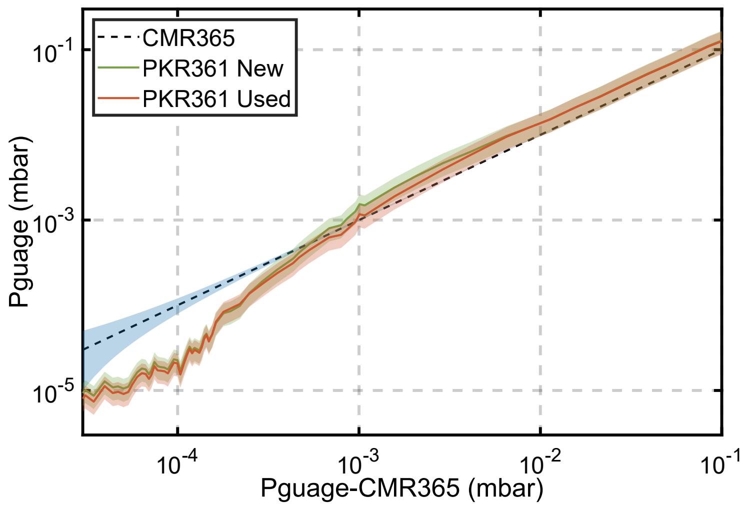


FIG. S1. Comparison of pressure readings between two cold cathode gauges and a capacitance gauge. The lines represent gauge readings taken during the measurement, while the shaded areas indicate the reading errors specified in the manufacturer's operating manual. Each data point is the average of 10 sets of measurement, which includes both the pressure-up and pressure-down processes.

Then, we averaged the acquired gauge signals and determined the reading errors in accordance with the instruction manual, where PKR361 exhibited a reading error of 30%, whereas CMR365 showed a reading of 0.5%. Additionally, CMR365 is subject to ambient temperature effects, resulting in a reading error of 0.03%/K and a zero poingt shift of 0.02%/K of its upper limit of measurement range. The temperature fluctuation in the experiment was ±1K.

As shown in the Fig. S1, there is almost no discrepancy between the used PKR361 and the new one. Compared to the capacitance gauge, the cold cathode gauge exhibited a slightly higher reading above $10^{-3}$ mbar, while remaining within the error given in the manufacturer's manual. However, the reading of the cold cathode gauge is significantly lower than that of the capacitance gauge below $10^{-3}$ mbar. Particular below $10^{-4}$ mbar, the reading is approximately 50% of that of the capacitance gauge, which is already a significant deviation from the manufacturer's indication error given for both cold cathode gauges. Nevertheless, these findings align with our results pertaining to the damping factor and air pressure measurements, which further supports the reliability of our approach.
